# Supplementary material for: Alpaka - An Abstraction Library for Parallel Kernel Acceleration
Source: arXiv:1602.08477 source file (2016-02-26)
Supplement: Supplementary file 1 [file appendix.tex]

\subsection{AXPY}

\begin{minipage}{\linewidth}
\hfill
\begin{lstlisting}[caption={Source code of sequential AXPY.}, label={lst:axpy_common}]
template<
    typename TSize,
    typename TElem>
auto axpy(
    TSize const & n,
    TElem const & alpha,
    TElem const * const X,
    TElem * const Y) const
-> void
{
  for(TSize i = 0; i < n; ++i)
  {
    Y[i] = alpha * X[i] + Y[i];
  }
}
\end{lstlisting}

\begin{lstlisting}[caption={Source code of CUDA AXPY function.}, label={lst:axpy_cuda}]

__global void axpy(
  const int n,
  const float alpha,
  const float *X,
  const float *Y)
{
  int i = blockDim.x*blockIdx.x+threadIdx;

  if(i < n)
  {
    Y[i] = alpha * X[i] + Y[i];
  }
}
  
\end{lstlisting}
\hfill
\end{minipage}

\begin{minipage}{\linewidth}
\hfill
\begin{lstlisting}[caption={Source code of \alpaka AXPY kernel functor with element extension.}, label={lst:axpy_alpaka_vec}]
struct Axpy{
  
  template<
    typename TAcc,
    typename TElem,
    typename TSize>
  ALPAKA_FN_ACC auto operator()(
    TAcc const & acc,
    TSize const & numElements,
    TElem const & alpha,
    TElem const * const X,
    TElem * const Y) const
  -> void
  {
    using namespace alpaka;
    
    TSize gridThreadIdx = idx::getIdx<Grid,Threads>(acc)[0u];
    
    TSize threadElemExtent = workdiv::getWorkDiv<Thread,Elems>(acc)[0u];
    
    TSize threadFirstElemIdx = gridThreadIdx*threadElemExtent;

    if(threadFirstElemIdx < numElements)
    {
      TSize elems = threadElemExtent + math::min(acc, 0, numElements - (threadFirstElemIdx + threadElemExtent));

      for(TSize i = threadFirstElemIdx; i < (threadFirstElemIdx + elems); ++i)
      {
        Y[i] = alpha * X[i] + Y[i];
      }
    }
  }
};
\end{lstlisting}
\hfill
\end{minipage}
